# Supplementary material for: Thinking Hard, Not Smart: Reasoning Models Fail to Ration Test-Time Compute Across Questions
Source: arXiv:2608.07968 source file (2026-08-11)
Supplement: Supplementary file 1 [file appendix.tex]

\appendix
\section{Detailed LLM Prompts}
\label{append:Prompts}

\input{img_tab_tex/full_QA_prompt}




% \section{Explicit Guidance on Test Taking Strategies}
% \label{append:explicit_guidance_prompts}
% We prompt the model with three different common human test-taking strategies, namely:
% \begin{itemize}
%     \item Explicit Plan: The model is instructed to explicitly plan its spending of the given budget to maximize total score.
%     \item Skipping: The model is hinted to skip questions that are too difficult or token-consuming.
%     \item Recheck: The model is instructed to double-check previous answers when there's ample budget.
% \end{itemize}

% The given prompts are:
% \input{img_tab_tex/explicit_plan_prompt}
% \input{img_tab_tex/skip_question_prompt}
% \input{img_tab_tex/recheck_answer_prompt}




\input{img_tab_tex/LLM_judge_prompt}
